# Supplementary material for: Reactive Task Allocation and Planning for Quadrupedal and Wheeled Robot Teaming
Source: arXiv:2110.08436 source file (2022-06-21)
Supplement: Supplementary file 1 [file appendix.tex]

\newpage
\section*{Appendix}
Proofs are elaborated in this section to complete our discussion in Sec.~\ref{reallocation_approach}.
\begin{proposition-1*}
The global specification will be fulfilled if a path is found by Algorithm 1 on the local PA $\mathcal{P}^{(r)}$ and all agents successfully accomplish their tasks.
\end{proposition-1*}

\begin{proof}
According to Algorithm 1 and the definition of $S_{c,\mathcal{P}}^{(r)}$, the newly found path 
\end{proof}

\begin{proposition-2*}
The global specification will be fulfilled if a path is found by Algorithm 2 on the revised local PA $\mathcal{P}^{(r)}(t)$ and all agents successfully accomplish their tasks.
\end{proposition-2*}

\begin{proof}
Algorithm 2 considers two 
\end{proof}

\begin{proposition-3*}
The synchronized team automaton preserves the properties of the original team automaton.
\end{proposition-3*}

\begin{proof}

\end{proof}
